# Supplementary material for: A time-dependent formulation of coupled cluster theory for many-fermion systems at finite temperature
Source: arXiv:1807.09961 ancillary file (2019-03-19)
Supplement: Supplementary file 1 [file supplemental.pdf]

# A time-dependent formulation of coupled cluster theory for many-fermion systems at finite temperature: Supplementary material

Alec F. White[1] and Garnet Kin-Lic Chan[1]

*Division of Chemistry and Chemical Engineering, California Institute of Technology, Pasadena, California 91125, USA*

(Dated: 11 March 2019)

Supplementary material to accompany: "A time-dependent formulation of coupled cluster theory for many-fermion systems at finite temperature" by Alec F. White and Garnet Chan. This supplement includes the complete set of results discussed in the aforementioned manuscript.

In the following sections we show FT-CCSD results for the unpolarized UEG. Table I shows the parameters used in these calculations. Calculations were performed at reduced temperatures ($\theta$) of 0.25, 0.5, and 1.

| $r_s$ | $L$ ($N = 14$) | $L$ ($N = 38$) | $L$ ($N = 66$) | $E_{\mathrm{F}}$ |
|---|---|---|---|---|
| 0.5 | 1.94256 | 2.70974 | 3.25722 | 7.36634 |
| 1.0 | 3.88513 | 5.41948 | 6.51445 | 1.84158 |
| 2.0 | 7.77026 | 10.83895 | 13.02889 | 0.46040 |
| 3.0 | 11.65539 | 16.25843 | 19.54334 | 0.20462 |
| 4.0 | 15.54052 | 21.67791 | 26.05779 | 0.11510 |

TABLE I. Box length ($L$) and Fermi energy ($E_{\mathrm{F}}$) for different numbers of electrons. Lengths are in units of Bohr ($a_0$) and energies are in units of Hartree ($E_{\mathrm{h}}$).

## I. $N = 14$ UNPOLARIZED UEG

- Results in a basis of 33 plane waves are shown in Table II
- Results in a basis of 57 plane waves are shown in Table III

## II. $N = 38$ UNPOLARLIZED UEG

- Results in a basis of 33 plane waves are shown in Table IV
- Results in a basis of 57 plane waves are shown in Table V
- A comparison of $E_{\mathrm{xc}}$ for different numbers of grid points is given in Table VI

## III. $N = 66$ UNPOLARIZED UEG

- Results in a basis of 57 plane waves are shown in Table VII

| $r_s$ | $\theta$ | $\mu_0$ | $\Omega_0$ | $E_0$ | $S_0$ |
|---|---|---|---|---|---|
| 0.5 | 1.00 | 1.54818 | -122.15842 | 130.34735 | 31.33597 |
| 0.5 | 0.50 | 5.53128 | -69.89354 | 103.56949 | 26.07132 |
| 0.5 | 0.25 | 7.01354 | -49.21035 | 81.31564 | 17.55904 |
| 1.0 | 1.00 | 0.38704 | -30.53961 | 32.58684 | 31.33597 |
| 1.0 | 0.50 | 1.38282 | -17.47338 | 25.89237 | 26.07132 |
| 1.0 | 0.25 | 1.75338 | -12.30259 | 20.32891 | 17.55904 |
| 2.0 | 1.00 | 0.09676 | -7.63490 | 8.14671 | 31.33597 |
| 2.0 | 0.50 | 0.34571 | -4.36835 | 6.47309 | 26.07132 |
| 2.0 | 0.25 | 0.43835 | -3.07565 | 5.08223 | 17.55904 |
| 3.0 | 1.00 | 0.04300 | -3.39329 | 3.62076 | 31.33597 |
| 3.0 | 0.50 | 0.15365 | -1.94149 | 2.87693 | 26.07132 |
| 3.0 | 0.25 | 0.19482 | -1.36695 | 2.25877 | 17.55904 |
| 4.0 | 1.00 | 0.02419 | -1.908738 | 2.03668 | 31.33597 |
| 4.0 | 0.50 | 0.08643 | -1.09209 | 1.61827 | 26.07132 |
| 4.0 | 0.25 | 0.10959 | -0.76891 | 1.27056 | 17.55904 |

| $r_s$ | $\theta$ | $N$ | $\mu_{\text{xc}}$ | $\Omega$ | $E_{\text{xc}}$ | $S_{\text{xc}}$ | $F_{\text{xc}}$ |
|---|---|---|---|---|---|---|---|
| 0.5 | 1.00 | 14.00001 | -0.47713 | -129.24841 | -1.04187 | -0.00792 | -0.98355 |
| 0.5 | 0.50 | 14.00001 | -0.53566 | -76.78353 | -1.08926 | -0.01668 | -1.02780 |
| 0.5 | 0.25 | 13.99998 | -0.57186 | -56.01356 | -1.07980 | -0.01194 | -1.05781 |
| 1.0 | 1.00 | 13.99953 | -0.24864 | -34.05726 | -0.53504 | -0.01903 | -0.49999 |
| 1.0 | 0.50 | 13.99348 | -0.28082 | -20.89475 | -0.55883 | -0.03577 | -0.52590 |
| 1.0 | 0.25 | 13.99808 | -0.29738 | -15.70717 | -0.55094 | -0.02218 | -0.54072 |
| 2.0 | 1.00 | 14.00000 | -0.13241 | -9.37587 | -0.27807 | -0.04628 | -0.25677 |
| 2.0 | 0.50 | 14.00000 | -0.14875 | -6.07905 | -0.28761 | -0.07240 | -0.27094 |
| 2.0 | 0.25 | 14.00001 | -0.15595 | -4.78192 | -0.28194 | -0.03568 | -0.27783 |
| 3.0 | 1.00 | 14.00000 | -0.09233 | -4.54616 | -0.18980 | -0.07392 | -0.17468 |
| 3.0 | 0.50 | 14.00009 | -0.10240 | -3.08213 | -0.19344 | -0.09349 | -0.18387 |
| 3.0 | 0.25 | 13.99999 | -0.10584 | -2.50724 | -0.18857 | -0.02517 | -0.18729 |
| 4.0 | 1.00 | 14.00000 | -0.07142 | -2.77043 | -0.14410 | -0.09672 | -0.13297 |
| 4.0 | 0.50 | 14.00000 | -0.07759 | -1.95270 | -0.14437 | -0.09226 | -0.13906 |
| 4.0 | 0.25 | 14.00000 | -0.07832 | -1.63769 | -0.13968 | 0.02396 | -0.14037 |

TABLE II. FT-CCSD results for the $N = 14$ systems using a basis of 33 plane waves. The exchange correlation contributions to extensive quantities ($E$, $S$, $F$) are given on a per-electron basis.

| $r_s$ | $\theta$ | $\mu_0$ | $\Omega_0$ | $E_0$ | $S_0$ |
|---|---|---|---|---|---|
| 0.5 | 1.00 | 0.46990 | -118.49764 | 153.2166 | 35.99288 |
| 0.5 | 0.50 | 5.45425 | -69.46127 | 106.54681 | 27.05512 |
| 0.5 | 0.25 | 7.01303 | -49.20598 | 81.34203 | 17.57484 |
| 1.0 | 1.00 | 0.11747 | -29.62441 | 38.30415 | 35.99288 |
| 1.0 | 0.50 | 1.36356 | -17.36532 | 26.6367 | 27.05512 |
| 1.0 | 0.25 | 1.75326 | -12.3015 | 20.33551 | 17.57484 |
| 2.0 | 1.00 | 0.02937 | -7.4061 | 9.57604 | 35.99288 |
| 2.0 | 0.50 | 0.34089 | -4.34133 | 6.65918 | 27.05512 |
| 2.0 | 0.25 | 0.43831 | -3.07537 | 5.08388 | 17.57484 |
| 3.0 | 1.00 | 0.01305 | -3.2916 | 4.25602 | 35.99288 |
| 3.0 | 0.50 | 0.15151 | -1.92948 | 2.95963 | 27.05512 |
| 3.0 | 0.25 | 0.19481 | -1.36683 | 2.25950 | 17.57484 |
| 4.0 | 1.00 | 0.00734 | -1.85153 | 2.39401 | 35.99288 |
| 4.0 | 0.50 | 0.08522 | -1.08533 | 1.66479 | 27.05512 |
| 4.0 | 0.25 | 0.10958 | -0.76884 | 1.27097 | 17.57484 |

| $r_s$ | $\theta$ | $N$ | $\mu_{\mathrm{xc}}$ | $\Omega$ | $E_{\mathrm{xc}}$ | $S_{\mathrm{xc}}$ | $F_{\mathrm{xc}}$ |
|---|---|---|---|---|---|---|---|
| 0.5 | 1.00 | 14.00000 | -0.45773 | -125.73694 | -1.06647 | -0.01244 | -0.97482 |
| 0.5 | 0.50 | 13.99993 | -0.54891 | -76.27280 | -1.10577 | -0.01909 | -1.03547 |
| 0.5 | 0.25 | 14.00000 | -0.58935 | -55.87733 | -1.08598 | -0.01091 | -1.06588 |
| 1.0 | 1.00 | 14.00001 | 0.17142 | -33.16842 | -0.55246 | -0.02863 | -0.49974 |
| 1.0 | 0.50 | 14.00001 | -0.23748 | -20.71539 | -0.56857 | -0.03887 | -0.53277 |
| 1.0 | 0.25 | 14.00000 | -0.29087 | -15.59981 | -0.55605 | -0.01893 | -0.54734 |
| 2.0 | 1.00 | 14.00001 | -0.13683 | -9.12557 | -0.28955 | -0.06495 | -0.25965 |
| 2.0 | 0.50 | 14.00000 | -0.15963 | -5.98109 | -0.29325 | -0.07163 | -0.27676 |
| 2.0 | 0.25 | 14.00009 | -0.16733 | -4.69111 | -0.28558 | -0.02467 | -0.28274 |
| 3.0 | 1.00 | 14.00006 | -0.09723 | -4.17480 | -0.18038 | -0.09807 | -0.16031 |
| 3.0 | 0.50 | 13.99993 | -0.11056 | -2.77294 | -0.17939 | -0.08387 | -0.17081 |
| 3.0 | 0.25 | 13.99998 | -0.11352 | -2.20306 | -0.17299 | 0.0052 | -0.17325 |
| 4.0 | 1.00 | 14.00000 | -0.07576 | -2.69000 | -0.14975 | -0.12255 | -0.13565 |
| 4.0 | 0.50 | 14.00000 | -0.08352 | -1.90782 | -0.14624 | -0.06899 | -0.14227 |
| 4.0 | 0.25 | 14.00000 | -0.08309 | -1.60185 | -0.15078 | 0.07965 | -0.15307 |

TABLE III. FT-CCSD results for the $N = 14$ systems using a basis of 57 plane waves. The exchange correlation contributions to extensive quantities ($E$, $S$, $F$) are given on a per-electron basis.

| $r_s$ | $\theta$ | $\mu_0$ | $\Omega_0$ | $E_0$ | $S_0$ |
|---|---|---|---|---|---|
| 0.5 | 1.00 | 8.68718 | -428.94107 | 223.90749 | 43.81225 |
| 0.5 | 0.50 | 7.63608 | -231.54239 | 208.79981 | 40.77229 |
| 0.5 | 0.25 | 7.16870 | -144.28309 | 188.55102 | 32.81067 |
| 1.0 | 1.00 | 2.17179 | -107.23527 | 55.97687 | 43.81225 |
| 1.0 | 0.50 | 1.90902 | -57.88560 | 52.19995 | 40.77229 |
| 1.0 | 0.25 | 1.79217 | -36.07077 | 47.13776 | 32.81067 |
| 2.0 | 1.00 | 0.54295 | -26.80882 | 13.99422 | 43.81225 |
| 2.0 | 0.50 | 0.47725 | -14.47140 | 13.04999 | 40.77229 |
| 2.0 | 0.25 | 0.44804 | -9.01769 | 11.78444 | 32.81067 |
| 3.0 | 1.00 | 0.24131 | -11.91503 | 6.21965 | 43.81225 |
| 3.0 | 0.50 | 0.21211 | -6.43173 | 5.79999 | 40.77229 |
| 3.0 | 0.25 | 0.19913 | -4.00786 | 5.23753 | 32.81067 |
| 4.0 | 1.00 | 0.13574 | -6.70220 | 3.49855 | 43.81225 |
| 4.0 | 0.50 | 0.11931 | -3.61785 | 3.2625 | 40.77229 |
| 4.0 | 0.25 | 0.11201 | -2.25442 | 2.94611 | 32.81067 |

| $r_s$ | $\theta$ | $N$ | $\mu_{\text{xc}}$ | $\Omega$ | $E_{\text{xc}}$ | $S_{\text{xc}}$ | $F_{\text{xc}}$ |
|---|---|---|---|---|---|---|---|
| 0.5 | 1.00 | 38.00169 | -0.74018 | -435.77884 | -0.95036 | -0.00400 | -0.92089 |
| 0.5 | 0.50 | 38.00018 | -0.74708 | -239.12781 | -0.99078 | -0.01196 | -0.94674 |
| 0.5 | 0.25 | 38.00257 | -0.7557 | -152.68730 | -1.01617 | -0.02113 | -0.97727 |
| 1.0 | 1.00 | 38.00033 | -0.36809 | -110.85823 | -0.48037 | -0.00918 | -0.46347 |
| 1.0 | 0.50 | 38.00124 | -0.36892 | -62.01985 | -0.50128 | -0.02551 | -0.47779 |
| 1.0 | 0.25 | 38.00055 | -0.37117 | -40.70841 | -0.51177 | -0.04025 | -0.49324 |
| 2.0 | 1.00 | 38.00037 | -0.18206 | -28.79665 | -0.24439 | -0.02175 | -0.23438 |
| 2.0 | 0.50 | 38.00060 | -0.18114 | -16.79657 | -0.25453 | -0.05293 | -0.24234 |
| 2.0 | 0.25 | 38.00022 | -0.18123 | -11.61620 | -0.25727 | -0.06649 | -0.24962 |
| 3.0 | 1.00 | 38.00025 | -0.12033 | -13.33656 | -0.16507 | -0.03580 | -0.15774 |
| 3.0 | 0.50 | 38.00038 | -0.11945 | -8.09489 | -0.17101 | -0.07609 | -0.16322 |
| 3.0 | 0.25 | 38.00232 | -0.11961 | -5.82033 | -0.17058 | -0.06392 | -0.16731 |
| 4.0 | 1.00 | 38.00160 | -0.08967 | -7.82617 | -0.12501 | -0.04997 | -0.11925 |
| 4.0 | 0.50 | 38.00058 | -0.08923 | -4.91068 | -0.12837 | -0.08889 | -0.12326 |
| 4.0 | 0.25 | 38.00241 | -0.09056 | -3.57166 | -0.12494 | 0.01010 | -0.12523 |

TABLE IV. FT-CCSD results for the $N = 38$ systems using a basis of 33 plane waves. The exchange correlation contributions to extensive quantities ($E$, $S$, $F$) are given on a per-electron basis.

| $r_s$ | $\theta$ | $\mu_0$ | $\Omega_0$ | $E_0$ | $S_0$ |
|---|---|---|---|---|---|
| 0.5 | 1.00 | 3.88076 | -356.43136 | 296.93302 | 68.67669 |
| 0.5 | 0.50 | 6.14411 | -202.00985 | 249.36359 | 59.16029 |
| 0.5 | 0.25 | 6.93722 | -138.19321 | 197.79797 | 39.30133 |
| 1.0 | 1.00 | 0.97019 | -89.10784 | 74.23326 | 68.67669 |
| 1.0 | 0.50 | 1.53603 | -50.50246 | 62.34089 | 59.16029 |
| 1.0 | 0.25 | 1.73431 | -34.54830 | 49.44949 | 39.30133 |
| 2.0 | 1.00 | 0.24255 | -22.27696 | 18.55831 | 68.67669 |
| 2.0 | 0.50 | 0.38401 | -12.62562 | 15.58523 | 59.16029 |
| 2.0 | 0.25 | 0.43358 | -8.63708 | 12.36237 | 39.30133 |
| 3.0 | 1.00 | 0.10780 | -9.90087 | 8.2484 | 68.67669 |
| 3.0 | 0.50 | 0.17067 | -5.61139 | 6.92677 | 59.16029 |
| 3.0 | 0.25 | 0.19270 | -3.83870 | 5.49439 | 39.30133 |
| 4.0 | 1.00 | 0.06064 | -5.56924 | 4.63958 | 68.67669 |
| 4.0 | 0.50 | 0.09600 | -3.15640 | 3.89631 | 59.16029 |
| 4.0 | 0.25 | 0.10839 | -2.15927 | 3.09059 | 39.30133 |

| $r_s$ | $\theta$ | $N$ | $\mu_{\text{xc}}$ | $\Omega$ | $E_{\text{xc}}$ | $S_{\text{xc}}$ | $F_{\text{xc}}$ |
|---|---|---|---|---|---|---|---|
| 0.5 | 1.00 | 38.00001 | -0.63707 | -365.29651 | -0.93755 | -0.00912 | -0.87036 |
| 0.5 | 0.50 | 38.00000 | -0.69329 | -210.94250 | -1.02318 | -0.02574 | -0.92836 |
| 0.5 | 0.25 | 38.00000 | -0.75023 | -147.16874 | -1.04795 | -0.03341 | -0.98643 |
| 1.0 | 1.00 | 37.99997 | -0.32506 | -93.63083 | -0.48345 | -0.02137 | -0.44409 |
| 1.0 | 0.50 | 38.00000 | -0.35244 | -55.19578 | -0.52473 | -0.05298 | -0.47595 |
| 1.0 | 0.25 | 38.00000 | -0.37615 | -39.39539 | -0.53068 | -0.05859 | -0.50370 |
| 2.0 | 1.00 | 38.00001 | -0.16760 | -24.61661 | -0.25214 | -0.04988 | -0.22917 |
| 2.0 | 0.50 | 38.00000 | -0.18038 | -15.12482 | -0.26975 | -0.10254 | -0.24615 |
| 2.0 | 0.25 | 38.00000 | -0.18969 | -11.24563 | -0.26933 | -0.09551 | -0.25833 |
| 3.0 | 1.00 | 38.00000 | -0.11437 | -11.49646 | -0.17239 | -0.07837 | -0.15636 |
| 3.0 | 0.50 | 38.00000 | -0.12263 | -7.31059 | -0.18140 | -0.13735 | -0.16735 |
| 3.0 | 0.25 | 38.00000 | -0.12932 | -5.53835 | -0.17903 | -0.09737 | -0.17405 |
| 4.0 | 1.00 | 38.00000 | -0.08739 | -6.78068 | -0.13106 | -0.10240 | -0.11927 |
| 4.0 | 0.50 | 37.99992 | -0.09351 | -4.41790 | -0.13511 | -0.14602 | -0.12670 |
| 4.0 | 0.25 | 38.00000 | -0.09895 | -3.32398 | -0.12851 | 0.03800 | -0.12960 |

TABLE V. FT-CCSD results for the $N = 38$ systems using a basis of 57 plane waves. The exchange correlation contributions to extensive quantities ($E$, $S$, $F$) are given on a per-electron basis.

| $r_s$ | $\theta$ | $E_{\text{xc}}$ ($n_g = 10$) | $E_{\text{xc}}$ ($n_g = 20$) | difference | % Absolute difference |
|---|---|---|---|---|---|
| 0.5 | 1.00 | -0.93755 | -0.93755 | 2.44E-06 | 0.00026 |
| 0.5 | 0.50 | -1.02318 | -1.02319 | 6.18E-06 | 0.00060 |
| 0.5 | 0.25 | -1.04795 | -1.04776 | 1.97E-04 | 0.01884 |
| 1.0 | 1.00 | -0.48345 | -0.48345 | 2.97E-06 | 0.00061 |
| 1.0 | 0.50 | -0.52473 | -0.52492 | 1.86E-04 | 0.03542 |
| 1.0 | 0.25 | -0.53068 | -0.53086 | 1.87E-04 | 0.03526 |
| 2.0 | 1.00 | -0.25214 | -0.25214 | 3.01E-06 | 0.00119 |
| 2.0 | 0.50 | -0.26975 | -0.26977 | 1.52E-05 | 0.00565 |
| 2.0 | 0.25 | -0.26933 | -0.26918 | 1.46E-04 | 0.05434 |
| 3.0 | 1.00 | -0.17239 | -0.17240 | 1.80E-06 | 0.00104 |
| 3.0 | 0.50 | -0.18140 | -0.18140 | 2.53E-06 | 0.00140 |
| 3.0 | 0.25 | -0.17903 | -0.17881 | 2.15E-04 | 0.12050 |
| 4.0 | 1.00 | -0.13106 | -0.13106 | 8.87E-07 | 0.00068 |
| 4.0 | 0.50 | -0.13511 | -0.13509 | 1.60E-05 | 0.01182 |
| 4.0 | 0.25 | -0.12851 | -0.12834 | 1.65E-04 | 0.12826 |

TABLE VI. Comparison of the exchange correlation energy of the $N = 38$ system (basis of 57 plane waves) for different numbers of grid points ($n_g = 10, 20$). Note that small differences can be caused by slightly different values of $N$ in the two calculations.

| $r_s$ | $\theta$ | $\mu_0$ | $\Omega_0$ | $E_0$ | $S_0$ |
|---|---|---|---|---|---|
| 0.5 | 1.00 | 8.90882 | -748.07967 | 396.83575 | 75.60521 |
| 0.5 | 0.50 | 7.85541 | -406.71917 | 371.16323 | 70.43536 |
| 0.5 | 0.25 | 7.52685 | -265.01795 | 335.80688 | 56.50163 |
| 1.0 | 1.00 | 2.2272 | -187.01992 | 99.20894 | 75.60521 |
| 1.0 | 0.50 | 1.96385 | -101.67979 | 92.79081 | 70.43536 |
| 1.0 | 0.25 | 1.88171 | -66.25449 | 83.95172 | 56.50163 |
| 2.0 | 1.00 | 0.55680 | -46.75498 | 24.80223 | 75.60521 |
| 2.0 | 0.50 | 0.49096 | -25.41995 | 23.1977 | 70.43536 |
| 2.0 | 0.25 | 0.47043 | -16.56362 | 20.98793 | 56.50163 |
| 3.0 | 1.00 | 0.24747 | -20.77999 | 11.02322 | 75.60521 |
| 3.0 | 0.50 | 0.21821 | -11.29775 | 10.31009 | 70.43536 |
| 3.0 | 0.25 | 0.20908 | -7.36161 | 9.32797 | 56.50163 |
| 4.0 | 1.00 | 0.13920 | -11.68874 | 6.20056 | 75.60521 |
| 4.0 | 0.50 | 0.12274 | -6.35499 | 5.79943 | 70.43536 |
| 4.0 | 0.25 | 0.11761 | -4.14091 | 5.24698 | 56.50163 |

| $r_s$ | $\theta$ | $N$ | $\mu_{\rm xc}$ | $\Omega$ | $E_{\rm xc}$ | $S_{\rm xc}$ | $F_{\rm xc}$ |
|---|---|---|---|---|---|---|---|
| 0.5 | 1.00 | 66.00000 | -0.80649 | -752.53959 | -0.90906 | -0.00475 | -0.87406 |
| 0.5 | 0.50 | 66.00000 | -0.80218 | -413.50998 | -0.95860 | -0.01453 | -0.90507 |
| 0.5 | 0.25 | 66.00000 | -0.78534 | -275.42550 | -0.99307 | -0.02717 | -0.94303 |
| 1.0 | 1.00 | 66.00000 | -0.39987 | -189.74859 | -0.46138 | -0.01095 | -0.44121 |
| 1.0 | 0.50 | 66.00002 | -0.39542 | -105.82407 | -0.48611 | -0.03030 | -0.45821 |
| 1.0 | 0.25 | 66.00001 | -0.38666 | -72.19868 | -0.49979 | -0.05009 | -0.47673 |
| 2.0 | 1.00 | 66.00004 | -0.19717 | -48.52772 | -0.23575 | -0.02546 | -0.22403 |
| 2.0 | 0.50 | 66.00004 | -0.19362 | -28.02931 | -0.24700 | -0.06015 | -0.23315 |
| 2.0 | 0.25 | 66.00000 | -0.18883 | -20.03692 | -0.25124 | -0.08506 | -0.24145 |
| 3.0 | 1.00 | 66.00000 | -0.13001 | -22.17578 | -0.15953 | -0.04088 | -0.15116 |
| 3.0 | 0.50 | 66.00000 | -0.12732 | -13.27629 | -0.16602 | -0.08529 | -0.15730 |
| 3.0 | 0.25 | 65.99997 | -0.12312 | -9.93332 | -0.16785 | -0.11269 | -0.16209 |
| 4.0 | 1.00 | 66.00000 | -0.09671 | -12.86188 | -0.12319 | -0.05604 | -0.11674 |
| 4.0 | 0.50 | 65.99996 | -0.09488 | -7.94608 | -0.12433 | -0.10445 | -0.11831 |
| 4.0 | 0.25 | 66.00000 | -0.09110 | -6.18257 | -0.12293 | -0.13972 | -0.11891 |

TABLE VII. FT-CCSD results for the $N = 66$ systems using a basis of 57 plane waves. The exchange correlation contributions to extensive quantities ($E$, $S$, $F$) are given on a per-electron basis.
